# Supplementary material for: Convergence of the Preconditioned Proximal Point Method and Douglas-Rachford Splitting in the Absence of Monotonicity
Source: arXiv:2305.03605 source file (2024-05-06)
Supplement: Supplementary file 1 [file matrix.tex]

%!TEX root = ../../../DRS-Minty.tex

\begin{definition}[Similarity] 
    \cite[Def. 1.3.1]{horn2012matrix}
    Let $A, B \in \R^{n \times n}$. $A$ is said to be similar to $B$ if there exists a nonsingular matrix $S \in \R^{n \times n}$ such that
    \[
        B = S^{-1} A S.
    \]
    The transformation $A \rightarrow S^{-1} A S$ is called a similarity transformation by the similarity matrix $S$. 
\end{definition}

\begin{proposition}
    \cite[Cor. 1.3.4]{horn2012matrix}
    If $A$ is similar to $B$, then $A$ and $B$ have the same eigenvalues.
\end{proposition}
